# Supplementary material for: Optimal Rates for Bandit Nonstochastic Control
Source: arXiv:2305.15352 source file (2023-10-25)
Supplement: Supplementary file 1 [file appendix-unknown.tex]

\section{Extension to Unknown Systems: Sketch}
\label{sec:control-unknown}
To control unknown systems, we engage in a two-part approach, where we first perform a system estimation and then engage in control under the assumption that the system is equal to that which we identified.

\subsubsection{Estimation of unknown Markov operator}
In the first part, we make use of the Markov operator estimation algorithm from \citep{simchowitz2020improper}. This estimation algorithm guarantees the low approximation error with high probability.
\begin{algorithm}
\caption{Estimation of Markov operator (Algorithm 2 in \citep{simchowitz2020improper})}
\label{alg:markov-est}
\begin{algorithmic}[1]
\STATE Input: Sample size $N$, system length $H$.
\STATE Initialize $\hat{G}^{[i]}=0$, $\forall i\notin[H]$. 
\FOR {$t = 1, \dots, N$}
\STATE Play action $\uv_t\sim N(0,I)$, observe $\y_{t+1}$.
\ENDFOR
\STATE Compute $\hat{G}^{[1:h]}\leftarrow \argmin \sum_{t=H+1}^T \left\|\y_t-\sum_{i=1}^H \hat{G}^{[i]}\uv_{t-i}\right\|_2^2$ via least squares. 
\STATE Return $\hat{G}$. 
\end{algorithmic}
\end{algorithm}

\begin{proposition} [Theorem 7 in \citep{simchowitz2020improper}] 
Let $\delta\in\left(e^{-T},T^{-1}\right)$, $N,d_{\uv}\le T$, $H$ satisfying $\sum_{n\ge H}\left\|G^{[n]}\right\|_{\mathrm{op}}\le\frac{1}{10}$. With probability at least $1-\delta-N^{-\log^2 N}$,
Algorithm~\ref{alg:markov-est} returns a $\hat{G}$ satisfying the following approximation error bound when $N\ge O(H^4C_{\delta}^4 R_{\M}^2R_G^2)$:
\begin{align*}
\sum_{n\ge 0}\|\hat{G}-G\|_{\mathrm{op}}\le \eps_G=O\left(\max\left\{R_{\M}R_G,\sqrt{d_{\uv}+2\log\left(\frac{3}{\delta}\right)}\right\}\right).
\end{align*}
\end{proposition}

\begin{lemma} [Lemma D.4 in \citep{simchowitz2020improper}]
$\|\hat{\ynat_t}-\ynat_t\|_2\le 2R_{\M}R\eps_G$. 
\end{lemma}
