# Supplementary material for: Optimal Rates for Bandit Nonstochastic Control
Source: arXiv:2305.15352 source file (2023-10-25)
Supplement: Supplementary file 2 [file appendix.tex]

\section{Expected strong convexity in the semi-adversarial noise model}

In this section we provide an alternate proof that the conditions of Corollary \ref{cor:regret-expected-convex} hold for the cost functions of LQR in the fully observed setting. The following Lemma is subsumed by
Corollary \ref{lem:expectation-strong-convex}, which applies more broadly to partially observed systems. However, it is self-contained and simple to prove, so we include it for convenience. 

\begin{lemma} 
Assume that $c_t(x,u) = x^\top Q x + u^\top R u$ is $\sigma$-strongly convex w.r.t. $u$. Let 
$$\ell_t(M) \defeq \E_{w}\left[c_t\left( x(M),u(M)  \right)\right],$$ 
be the expected loss as a function of DAC parameterization $M = M_1,...,M_H$, where the expectation is taken over the perturbations such that we have
$$ \E \sum_{ij} w_i w_j^\top  \succeq \tau I .$$
Then ${\ell}_t(M)$ is $\sigma'$-strongly convex in $M$ for $\sigma' = \sigma \times \tau $. 
\end{lemma}
\begin{proof}
By definition, $u(M) = \sum_i M w_i$, since we evaluate on $(M_1,...,M_H)=(M,...,M)$.
Using the chain rule for differentiation, 
\begin{align*}
\E\left[\nabla^2 \ell_t(M)\right] & = \E\left[\nabla^2 \left[ x(M)^\top Q x(M) + u(M)^\top R u(M) \right]\right] \\
& \succeq \E \left[\nabla^2  u(M)^\top R u(M)\right] & \mbox{convexity} \\
& = \E \left[\nabla^2 \left[ \left(\sum_i M w_{t-i}\right)^\top   R \left(\sum_i M w_{t-i}\right) \right]\right]  & \mbox{defn of $u$} \\
& =  \nabla^2  \sum_{ij}  \E  \left[ w_i^\top M   R  M w_j  \right]  & \mbox{linearity of expectation} \\
& =  \nabla^2      \left(MRM\right) \bullet  \sum_{ij} \E \left[ w_j w_i^\top  \right]  & x^\top A y = A \bullet x y^\top  \\
& \geq \nabla^2      \left(MRM\right) \bullet \tau I \\
& = \tau  \nabla^2  \trace \left(MRM\right)
\end{align*}
Next, we have that 
$$ \nabla \trace(MRM) = 2 MR  , $$
and thus 
$$ \nabla^2 MRM = 2 R \oplus R \succeq \tau I \oplus I  $$
\end{proof}
